# Supplementary material for: Machine Learning-Driven Structure Prediction for Iron Hydrides
Source: arXiv:2311.06010 source file (2023-11-10)
Supplement: Supplementary file 1 [file Supplemental_material.pdf]

# Supporting Information: Machine Learning-Driven Structure Prediction for Iron Hydrides

Hossein Tahmasbi,*,† Kushal Ramakrishna,† Mani Lokamani,‡ and Attila Cangi*,†

†*Center for Advanced Systems Understanding (CASUS), D-02826 Görlitz, Germany*

‡*Helmholtz-Zentrum Dresden-Rossendorf (HZDR), D-01328 Dresden, Germany*

E-mail: h.tahmasbi@hzdr.de; a.cangi@hzdr.de

This document provides structural data for some of the FeH structures discussed in the main manuscript. The atomic coordinates for these structures are listed in Cartesian coordinates in Section 1.1. Section 1.2 lists all the minima structures for FeH at different pressures that were found in this study. The phonon dispersions of select structures are provided in Section 2. Plots of the phase diagram, bulk modulus, and electrical conductivity are provided in Sections 3, 4, and 5, respectively.

# Contents


**1 Structural data of FeH** **S4**

1.1 Structural data for some phases . . . . . S4

1.2 Minima structures of FeH at different pressures . . . . . S8

1.2.1 P= 0 GPa . . . . . S8

1.2.2 P= 10 GPa . . . . . S9

1.2.3 P= 20 GPa . . . . . S10

1.2.4 P= 30 GPa . . . . . S10

1.2.5 P= 40 GPa . . . . . S11

1.2.6 P= 50 GPa . . . . . S11

1.2.7 P= 60 GPa . . . . . S12

1.2.8 P= 70 GPa . . . . . S12

1.2.9 P= 80 GPa . . . . . S13

1.2.10 P= 90 GPa . . . . . S14

1.2.11 P= 100 GPa . . . . . S14

**2 Phonon dispersion** **S15**

2.1 P= 0 GPa . . . . . S15

2.2 P= 10 GPa . . . . . S15

2.3 P= 20 GPa . . . . . . . . . . . . . . . . . . . . . . . . . . . . . . . . . . . S16

2.4 P= 30 GPa . . . . . . . . . . . . . . . . . . . . . . . . . . . . . . . . . . . S17

2.5 P= 40 GPa . . . . . . . . . . . . . . . . . . . . . . . . . . . . . . . . . . . S17

2.6 P= 50 GPa . . . . . . . . . . . . . . . . . . . . . . . . . . . . . . . . . . . S18

2.7 P= 60 GPa . . . . . . . . . . . . . . . . . . . . . . . . . . . . . . . . . . . S18

2.8 P= 70 GPa . . . . . . . . . . . . . . . . . . . . . . . . . . . . . . . . . . . S19

2.9 P= 80 GPa . . . . . . . . . . . . . . . . . . . . . . . . . . . . . . . . . . . S19

2.10 P= 90 GPa . . . . . . . . . . . . . . . . . . . . . . . . . . . . . . . . . . . S20

2.11 P= 100 GPa . . . . . . . . . . . . . . . . . . . . . . . . . . . . . . . . . . . S20

**3 Phase diagram** **S21**

**4 Bulk modulus** **S22**

**5 Electrical conductivity** **S23**

# 1 Structural data of FeH

## 1.1 Structural data for some phases

| Data for "hcp", "P 63/m 2/m 2/c"(194) at P = 0 GPa | | | |
|---|---|---|---|
| Unit cell dimensions | a = 2.64264 | b = 2.64264 | c = 4.33101 |
| | $\alpha$ = 90 | $\beta$ = 90 | $\gamma$ = 120 |
| Atom | x | y | z |
| Fe(1) | 0.33333 | 0.66667 | 0.75000 |
| H(1) | 0.00000 | 0.00000 | 0.00000 |

| Data for "dhcp", "P 63/m 2/m 2/c"(194) at P = 0 GPa | | | |
|---|---|---|---|
| Unit cell dimensions | a = 2.64944 | b = 2.64944 | c = 8.63435 |
| | $\alpha$ = 90 | $\beta$ = 90 | $\gamma$ = 120 |
| Atom | x | y | z |
| Fe(1) | 0.33333 | 0.66667 | 0.25000 |
| Fe(2) | 0.00000 | 0.00000 | 0.00000 |
| H(1) | 0.33333 | 0.66667 | 0.62019 |

| Data for "fcc", "F4/m-32/m"(225) at P = 0 GPa | | | |
|---|---|---|---|
| Unit cell dimensions | a = 3.76495 | b = 3.76495 | c = 3.76495 |
| | $\alpha$ = 90 | $\beta$ = 90 | $\gamma$ = 90 |
| Atom | x | y | z |
| Fe(1) | 0.000000 | 0.000000 | 0.000000 |
| H(1) | 0.500000 | 0.500000 | 0.500000 |

| Data for "N1", "R -3 2/m"(166) at P = 0 GPa | | | |
|---|---|---|---|
| Unit cell dimensions | a = 2.64899 | b = 2.64899 | c = 32.54575 |
| | $\alpha$ = 90 | $\beta$ = 90 | $\gamma$ = 120 |
| Atom | x | y | z |
| Fe(1) | 0.00000 | 0.00000 | 0.36626 |
| Fe(2) | 0.00000 | 0.00000 | 0.50000 |
| Fe(3) | 0.00000 | 0.00000 | 0.76703 |
| H(1) | 0.00000 | 0.00000 | 0.13484 |
| H(2) | 0.00000 | 0.00000 | 0.06647 |
| H(3) | 0.00000 | 0.00000 | 0.00000 |

| Data for "N2", "R -3 2/m"(166) at P = 0 GPa | | | |
|---|---|---|---|
| Unit cell dimensions | a = 2.65313 | b = 2.65313 | c = 19.50817 |
| | $\alpha = 90$ | $\beta = 90$ | $\gamma = 120$ |
| Atom | x | y | z |
| Fe(1) | 0.00000 | 0.00000 | 0.50000 |
| Fe(2) | 0.00000 | 0.00000 | 0.27706 |
| H(1) | 0.00000 | 0.00000 | 0.11354 |
| H(2) | 0.00000 | 0.00000 | 0.00000 |

| Data for "N3", "R -3 2/m"(166) at P = 0 GPa | | | |
|---|---|---|---|
| Unit cell dimensions | a = 2.64715 | b = 2.64715 | c = 39.05241 |
| | $\alpha = 90$ | $\beta = 90$ | $\gamma = 120$ |
| Atom | x | y | z |
| Fe(1) | 0.00000 | 0.00000 | 0.19436 |
| Fe(2) | 0.00000 | 0.00000 | 0.58339 |
| Fe(3) | 0.00000 | 0.00000 | 0.30575 |
| H(1) | 0.00000 | 0.00000 | -0.05531 |
| H(2) | 0.00000 | 0.00000 | 0.50000 |
| H(3) | 0.00000 | 0.00000 | 0.11183 |
| H(4) | 0.00000 | 0.00000 | 0.00000 |

| Data for "N4", "R -3 2/m"(166) at P = 0 GPa | | | |
|---|---|---|---|
| Unit cell dimensions | a = 2.65779 | b = 2.65779 | c = 26.04906 |
| | $\alpha = 90$ | $\beta = 90$ | $\gamma = 120$ |
| Atom | x | y | z |
| Fe(1) | 0.00000 | 0.00000 | 0.87529 |
| Fe(2) | 0.00000 | 0.00000 | 0.29184 |
| H(1) | 0.00000 | 0.00000 | 0.50000 |
| H(2) | 0.00000 | 0.00000 | 0.00000 |
| H(3) | 0.00000 | 0.00000 | 0.58463 |

| Data for "N5", "P -3 2/m 1"(164) at P = 0 GPa | | | |
|---|---|---|---|
| Unit cell dimensions | a = 2.65790 | b = 2.65790 | c = 10.84839 |
| | $\alpha = 90$ | $\beta = 90$ | $\gamma = 120$ |
| Atom | x | y | z |
| Fe(1) | 0.33333 | 0.66667 | 0.39914 |
| Fe(2) | 0.00000 | 0.00000 | 0.00000 |
| Fe(3) | 0.33333 | 0.66667 | 0.79983 |
| H(1) | 0.33333 | 0.66667 | 0.10130 |
| H(2) | 0.00000 | 0.00000 | 0.29651 |
| H(3) | 0.00000 | 0.00000 | 0.50000 |

| Data for “N6”, “R -3 2/m”(166) at P = 0 GPa | | | |
|---|---|---|---|
| Unit cell dimensions | a = 2.65841 | b = 2.65841 | c = 39.06706 |
| | $\alpha = 90$ | $\beta = 90$ | $\gamma = 120$ |
| Atom | x | y | z |
| Fe(1) | 0.00000 | 0.00000 | 0.58338 |
| Fe(2) | 0.00000 | 0.00000 | 0.69460 |
| Fe(3) | 0.00000 | 0.00000 | 0.86126 |
| H(1) | 0.00000 | 0.00000 | -0.05639 |
| H(2) | 0.00000 | 0.00000 | 0.22247 |
| H(3) | 0.00000 | 0.00000 | 0.00000 |
| H(4) | 0.00000 | 0.00000 | 0.50000 |

| Data for “S02 (N8)”, “P -6 m 2”(187) at P = 20 GPa | | | |
|---|---|---|---|
| Unit cell dimensions | a = 2.57663 | b = 2.57663 | c = 12.56800 |
| | $\alpha = 90$ | $\beta = 90$ | $\gamma = 120$ |
| Atom | x | y | z |
| Fe(1) | 0.33333 | 0.66667 | 0.50000 |
| Fe(2) | 0.66667 | 0.33333 | 0.83323 |
| Fe(3) | 0.00000 | 0.00000 | 0.66676 |
| Fe(4) | 0.00000 | 0.00000 | 0.00000 |
| H(1) | 0.33333 | 0.66667 | 0.74723 |
| H(2) | 0.33333 | 0.66667 | -0.08310 |
| H(3) | 0.66667 | 0.33333 | 0.58610 |

| Data for “S04”, “P -6 m 2”(187) at P = 20 GPa | | | |
|---|---|---|---|
| Unit cell dimensions | a = 2.57547 | b = 2.57547 | 16.79303 |
| | $\alpha = 90$ | $\beta = 90$ | $\gamma = 120$ |
| Atom | x | y | z |
| Fe(1) | 0.00000 | 0.00000 | 0.25010 |
| Fe(2) | 0.66667 | 0.33333 | 0.50000 |
| Fe(3) | 0.33333 | 0.66667 | 0.12484 |
| Fe(4) | 0.00000 | 0.00000 | 0.00000 |
| Fe(5) | 0.33333 | 0.66667 | 0.37488 |
| H(1) | 0.66667 | 0.33333 | 0.31455 |
| H(2) | 0.00000 | 0.00000 | 0.43539 |
| H(3) | 0.66667 | 0.33333 | -0.06250 |
| H(4) | 0.66667 | 0.33333 | 0.18737 |

| Data for "S05", "P 63/m 2/m 2/c"(194) at P = 20 GPa | | | |
|---|---|---|---|
| Unit cell dimensions | a = 2.57514 | b = 2.57514 | 16.78572 |
| | $\alpha = 90$ | $\beta = 90$ | $\gamma = 120$ |
| Atom | x | y | z |
| Fe(1) | 0.33333 | 0.66667 | 0.12493 |
| Fe(2) | 0.00000 | 0.00000 | 0.00000 |
| Fe(3) | 0.00000 | 0.00000 | 0.25000 |
| H(1) | 0.33333 | 0.66667 | 0.56052 |
| H(2) | 0.33333 | 0.66667 | 0.81239 |

| Data for "S11 (N7)", "P 63/m 2/m 2/c"(194) at P = 20 GPa | | | |
|---|---|---|---|
| Unit cell dimensions | a = 2.58273 | b = 2.58273 | c = 12.57520 |
| | $\alpha = 90$ | $\beta = 90$ | $\gamma = 120$ |
| Atom | x | y | z |
| Fe(1) | 0.33333 | 0.66667 | 0.41710 |
| Fe(2) | 0.00000 | 0.00000 | 0.25000 |
| H(1) | 0.33333 | 0.66667 | 0.66440 |
| H(2) | 0.00000 | 0.00000 | 0.00000 |

## 1.2 Minima structures of FeH at different pressures

### 1.2.1 P= 0 GPa

Table S1: Minima structures of FeH at P= 0 GPa

| Label | Space group | Phase | N | ΔE (eV/atom) |
|---|---|---|---|---|
| S01 | 194 | hcp | 16 | 0.000 |
| S02 | 194 | dhcp | 24 | 0.002 |
| S03 | 166 | N1 | 20 | 0.002 |
| S04 | 166 | N2 | 24 | 0.003 |
| S05 | 166 | | 20 | 0.004 |
| S06 | 166 | N3 | 36 | 0.004 |
| S07 | 164 | | 28 | 0.005 |
| S08 | 166 | N4 | 16 | 0.006 |
| S09 | 164 | N5 | 20 | 0.008 |
| S10 | 166 | N6 | 24 | 0.009 |
| S11 | 225 | fcc | 16 | 0.013 |
| S12 | 160 | | 28 | 0.021 |
| S13 | 156 | | 24 | 0.021 |
| S14 | 160 | | 36 | 0.022 |
| S15 | 160 | | 20 | 0.024 |
| S16 | 160 | | 20 | 0.025 |
| S17 | 160 | | 36 | 0.028 |
| S18 | 156 | | 16 | 0.029 |

### 1.2.2 P= 10 GPa

Table S2: Minima structures of FeH at P= 10 GPa

| Label | Space group | Phase | N | ΔH (eV/atom) |
|---|---|---|---|---|
| S01 | 194 | hcp | 16 | 0.000 |
| S02 | 166 | N1 | 20 | 0.002 |
| S03 | 194 | dhcp | 16 | 0.003 |
| S04 | 166 | | 28 | 0.003 |
| S05 | 166 | N2 | 36 | 0.004 |
| S06 | 166 | | 20 | 0.006 |
| S07 | 160 | | 20 | 0.006 |
| S08 | 160 | | 20 | 0.008 |
| S09 | 164 | | 28 | 0.008 |
| S10 | 166 | N4 | 16 | 0.009 |
| S11 | 166 | | 24 | 0.010 |
| S12 | 164 | N5 | 20 | 0.011 |
| S13 | 166 | | 20 | 0.013 |
| S14 | 166 | | 28 | 0.014 |
| S15 | 225 | fcc | 24 | 0.019 |

#### 1.2.3 P= 20 GPa

Table S3: Minima structures of FeH at P= 20 GPa

| Label | Space group | Phase | N | ΔH (eV/atom) |
|---|---|---|---|---|
| S01 | 194 | hcp | 16 | 0.000 |
| S02 | 187 | N8 | 24 | 0.003 |
| S03 | 166 | N1 | 20 | 0.003 |
| S04 | 187 | | 16 | 0.003 |
| S05 | 194 | | 16 | 0.003 |
| S06 | 194 | dhcp | 16 | 0.004 |
| S07 | 166 | N2 | 24 | 0.006 |
| S08 | 166 | | 20 | 0.010 |
| S09 | 166 | N4 | 24 | 0.011 |
| S10 | 166 | | 16 | 0.012 |
| S11 | 194 | N7 | 24 | 0.013 |
| S12 | 164 | | 20 | 0.014 |
| S13 | 166 | | 16 | 0.016 |
| S14 | 225 | fcc | 32 | 0.023 |

#### 1.2.4 P= 30 GPa

Table S4: Minima structures of FeH at P= 30 GPa

| Label | Space group | Phase | N | ΔH (eV/atom) |
|---|---|---|---|---|
| S01 | 194 | hcp | 16 | 0.000 |
| S02 | 166 | N1 | 20 | 0.003 |
| S03 | 194 | dhcp | 16 | 0.005 |
| S04 | 166 | N2 | 24 | 0.006 |
| S05 | 166 | N4 | 16 | 0.012 |
| S06 | 164 | | 20 | 0.016 |
| S07 | 225 | fcc | 36 | 0.027 |

#### 1.2.5 P= 40 GPa

Table S5: Minima structures of FeH at P= 40 GPa

| Label | Space group | Phase | N | ΔH (eV/atom) |
|---|---|---|---|---|
| S01 | 194 | hcp | 16 | 0.000 |
| S02 | 166 | N1 | 20 | 0.003 |
| S03 | 166 | N2 | 24 | 0.006 |
| S04 | 194 | dhcp | 16 | 0.006 |
| S05 | 160 | | 28 | 0.009 |
| S06 | 225 | fcc | 20 | 0.010 |
| S07 | 166 | N4 | 32 | 0.011 |
| S08 | 194 | N7 | 24 | 0.015 |

#### 1.2.6 P= 50 GPa

Table S6: Minima structures of FeH at P= 50 GPa

| Label | Space group | Phase | N | ΔH (eV/atom) |
|---|---|---|---|---|
| S01 | 225 | fcc | 16 | 0.000 |
| S02 | 194 | hcp | 16 | 0.001 |
| S03 | 164 | N5 | 20 | 0.003 |
| S04 | 166 | N1 | 20 | 0.004 |
| S05 | 166 | N2 | 36 | 0.005 |
| S06 | 187 | N8 | 24 | 0.007 |
| S07 | 194 | dhcp | 16 | 0.009 |

### 1.2.7 P= 60 GPa

Table S7: Minima structures of FeH at P= 60 GPa

| Label | Space group | Phase | N | ΔH (eV/atom) |
|---|---|---|---|---|
| S01 | 225 | fcc | 20 | 0.000 |
| S02 | 164 | N5 | 20 | 0.006 |
| S03 | 166 | N4 | 16 | 0.008 |
| S04 | 166 | N3 | 36 | 0.008 |
| S05 | 194 | hcp | 16 | 0.009 |
| S06 | 164 | | 28 | 0.010 |
| S07 | 166 | N2 | 24 | 0.012 |
| S08 | 166 | N1 | 20 | 0.012 |

### 1.2.8 P= 70 GPa

Table S8: Minima structures of FeH at P= 70 GPa

| Label | Space group | Phase | N | ΔH (eV/atom) |
|---|---|---|---|---|
| S01 | 225 | fcc | 16 | 0.000 |
| S02 | 166 | | 36 | 0.008 |
| S03 | 194 | dhcp | 24 | 0.009 |
| S04 | 164 | N5 | 20 | 0.009 |
| S05 | 166 | N4 | 16 | 0.011 |
| S06 | 166 | | 36 | 0.012 |
| S07 | 166 | N1 | 20 | 0.016 |
| S08 | 194 | hcp | 16 | 0.017 |
| S09 | 166 | N2 | 36 | 0.018 |

### 1.2.9 P= 80 GPa

Table S9: Minima structures of FeH at P= 80 GPa

| Label | Space group | Phase | N | ΔH (eV/atom) |
|---|---|---|---|---|
| S01 | 225 | fcc | 16 | 0.000 |
| S02 | 194 | N7 | 36 | 0.004 |
| S03 | 166 | | 24 | 0.006 |
| S04 | 166 | | 20 | 0.007 |
| S05 | 166 | N6 | 24 | 0.008 |
| S06 | 194 | dhcp | 24 | 0.009 |
| S07 | 164 | N5 | 20 | 0.009 |
| S08 | 166 | | 32 | 0.011 |
| S09 | 166 | N4 | 24 | 0.011 |
| S10 | 166 | N2 | 36 | 0.016 |
| S11 | 166 | N1 | 20 | 0.018 |
| S12 | 194 | hcp | 16 | 0.021 |

#### 1.2.10 P= 90 GPa

Table S10: Minima structures of FeH at P= 90 GPa

| Label | Space group | Phase | N | ΔH (eV/atom) |
|---|---|---|---|---|
| S01 | 225 | fcc | 16 | 0.000 |
| S02 | 194 | N7 | 36 | 0.004 |
| S03 | 166 | | 20 | 0.006 |
| S04 | 194 | dhcp | 24 | 0.008 |
| S05 | 164 | N5 | 20 | 0.009 |
| S06 | 166 | N4 | 32 | 0.011 |
| S07 | 166 | N3 | 36 | 0.015 |
| S08 | 166 | N2 | 36 | 0.015 |
| S09 | 166 | N1 | 20 | 0.019 |
| S10 | 194 | hcp | 32 | 0.024 |

#### 1.2.11 P= 100 GPa

Table S11: Minima structures of FeH at P= 100 GPa

| Label | Space group | Phase | N | ΔH (eV/atom) |
|---|---|---|---|---|
| S01 | 225 | fcc | 16 | 0.000 |
| S02 | 166 | | 24 | 0.007 |
| S03 | 166 | | 20 | 0.008 |
| S04 | 194 | dhcp | 24 | 0.010 |
| S05 | 164 | N5 | 20 | 0.011 |
| S06 | 166 | N4 | 24 | 0.013 |
| S07 | 166 | N2 | 24 | 0.018 |
| S08 | 166 | N1 | 20 | 0.022 |
| S09 | 194 | hcp | 28 | 0.028 |

# 2 Phonon dispersion

## 2.1 P= 0 GPa

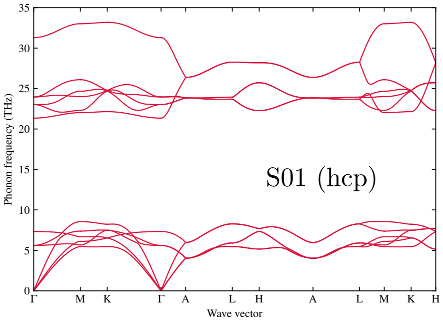


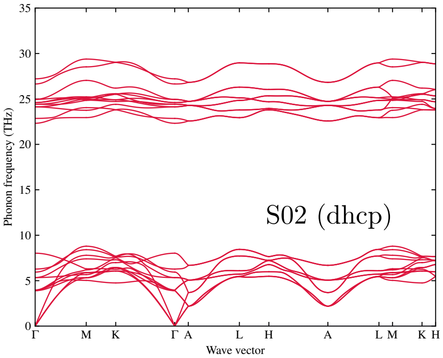


## 2.2 P= 10 GPa

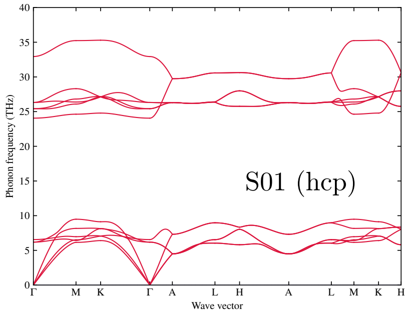


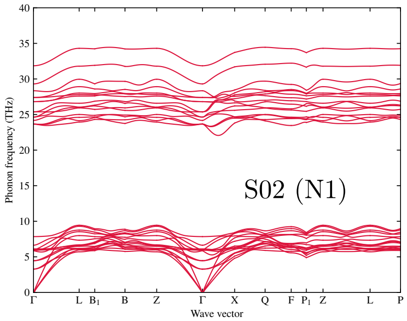


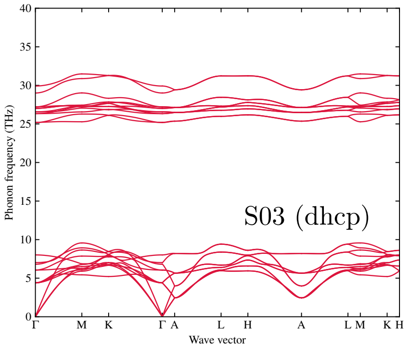


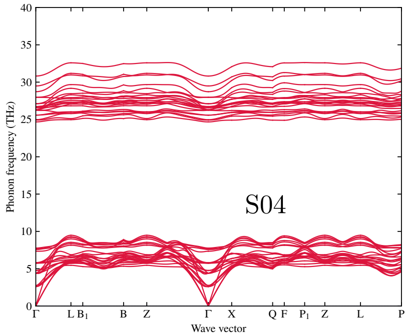


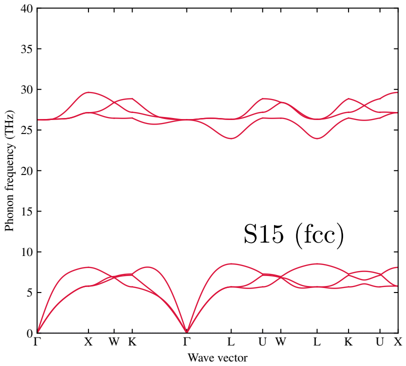

## 2.3 P= 20 GPa

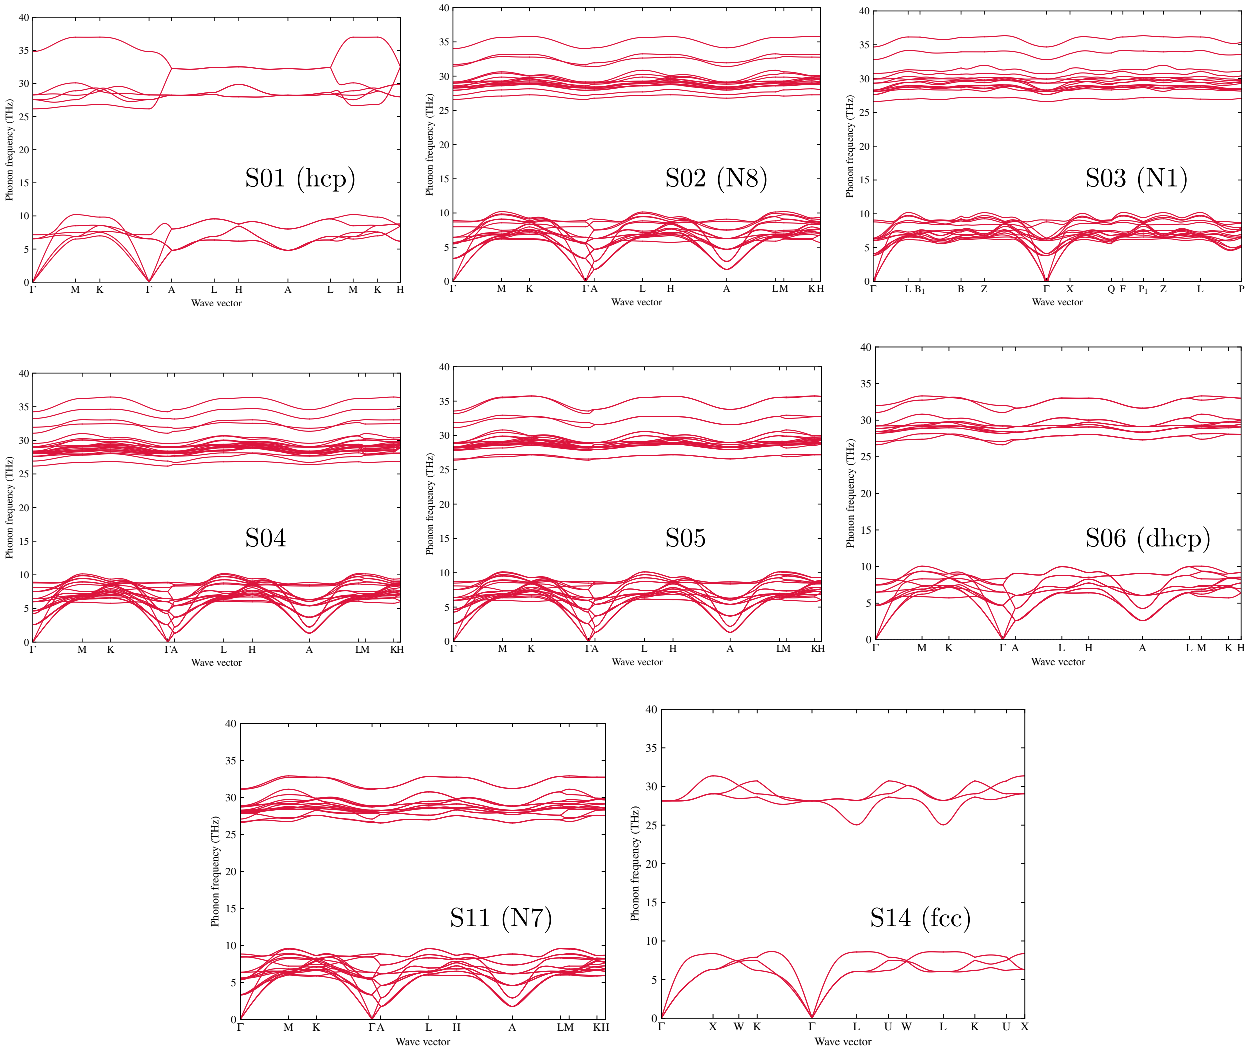
S01 (hcp)
S02 (N8)
S03 (N1)
S04
S05
S06 (dhcp)
S11 (N7)
S14 (fcc)
Phonon frequency (THz)
Wave vector

## 2.4 P= 30 GPa

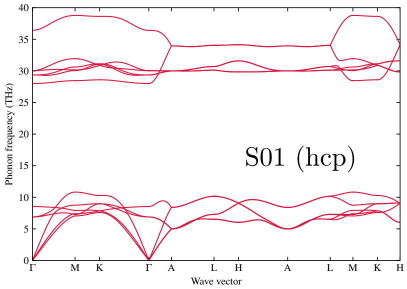


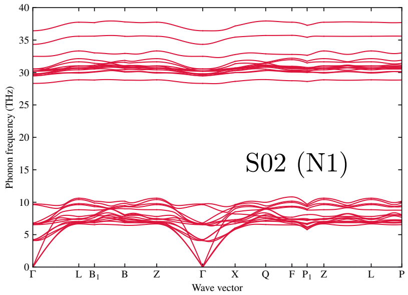


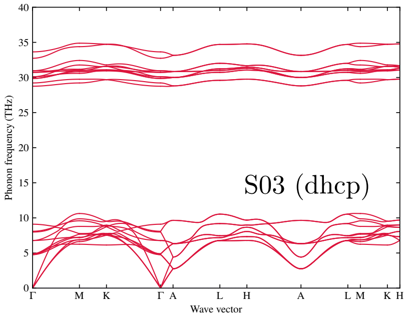


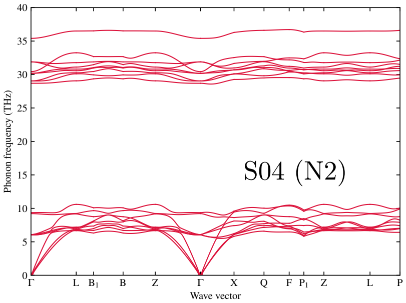


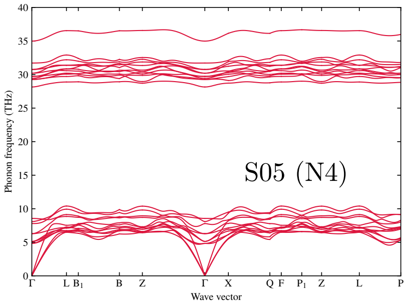


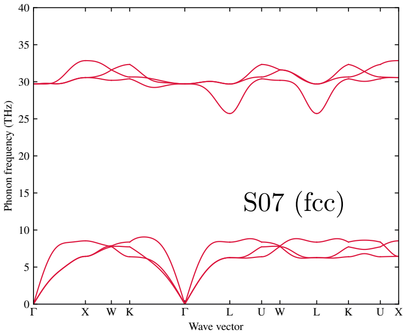


## 2.5 P= 40 GPa

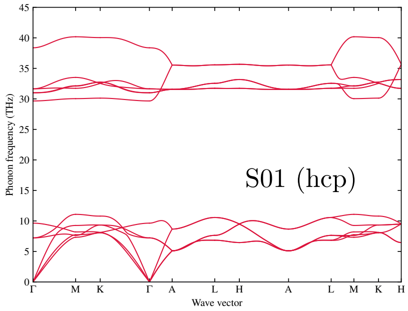


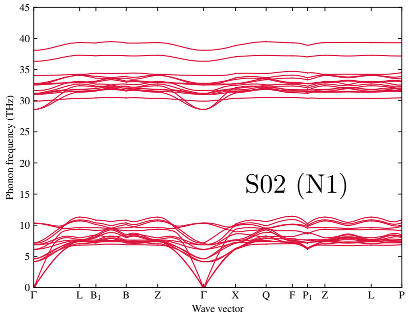


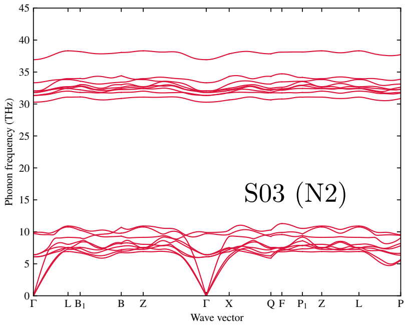


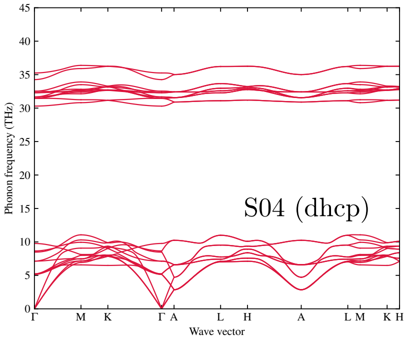

## 2.6 P= 50 GPa

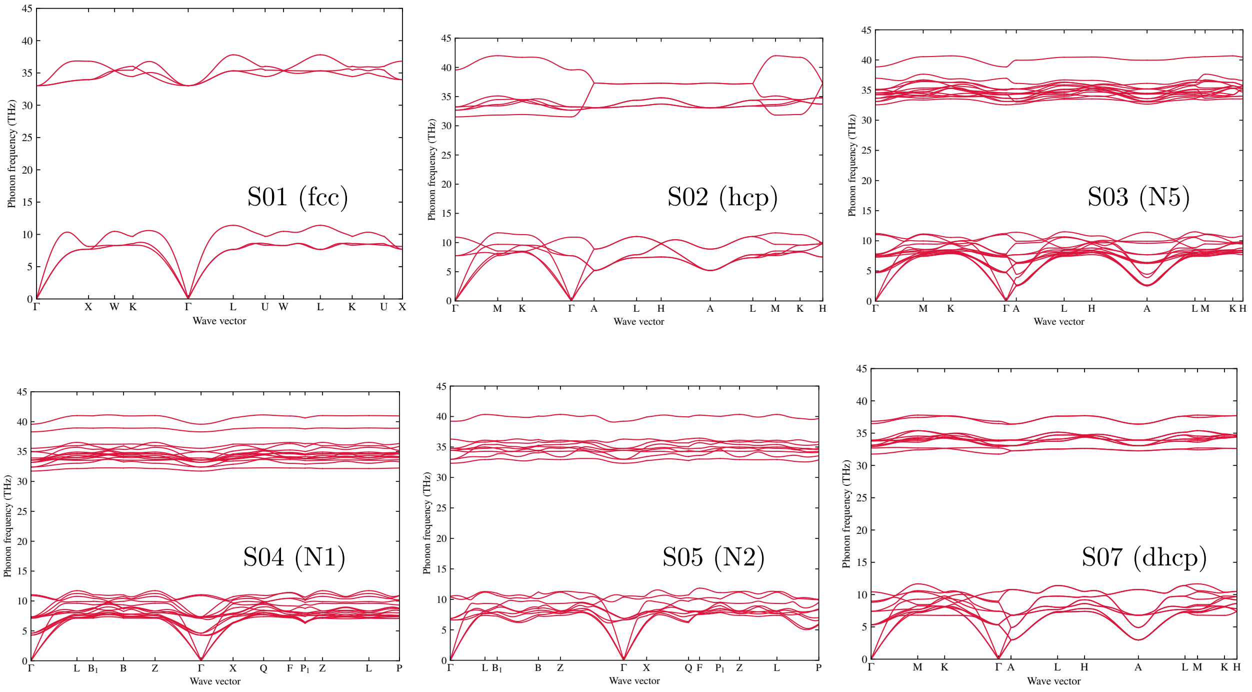


## 2.7 P= 60 GPa

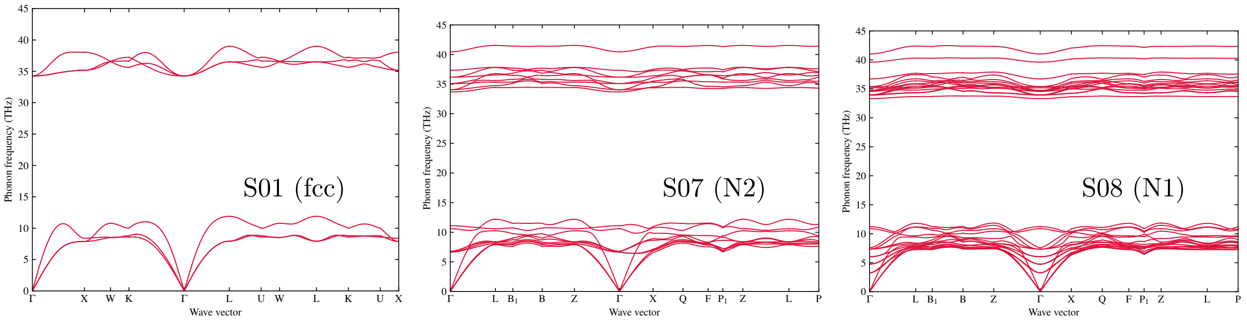

## 2.8 P= 70 GPa

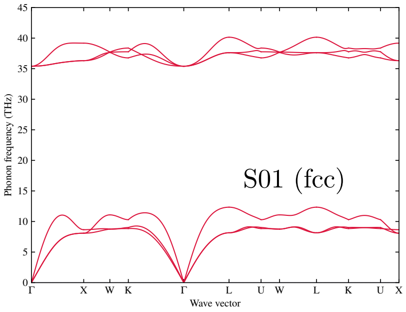


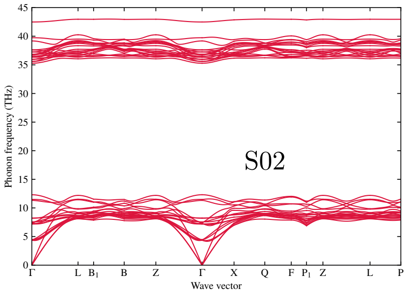


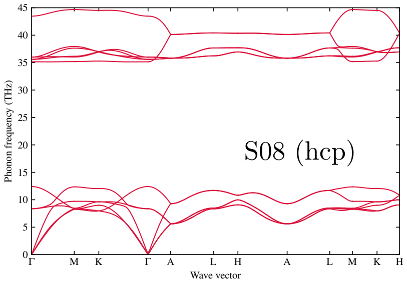


## 2.9 P= 80 GPa

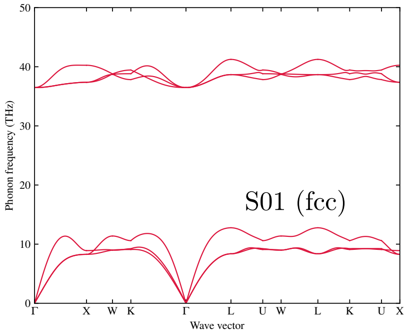


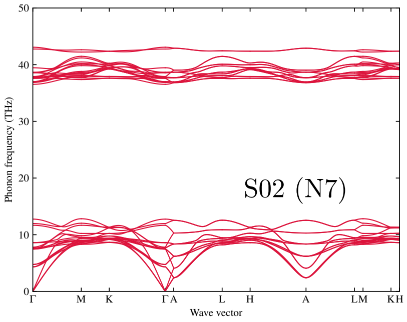


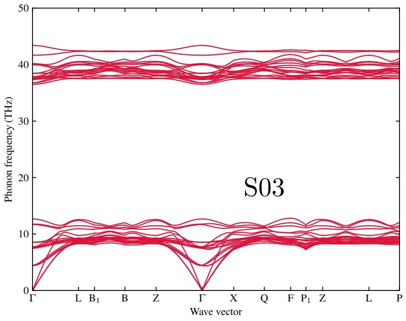


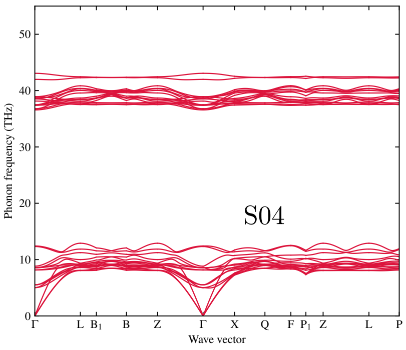


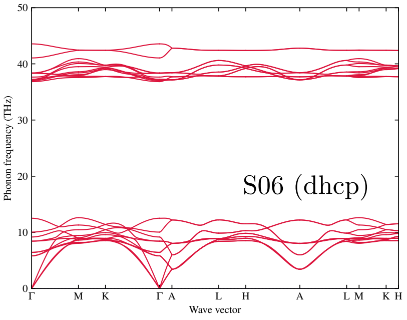


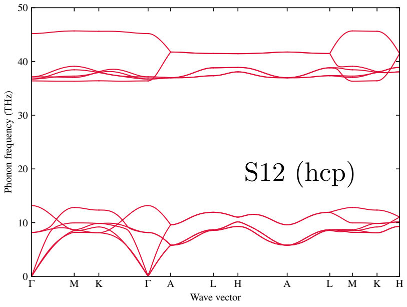

## 2.10 P= 90 GPa

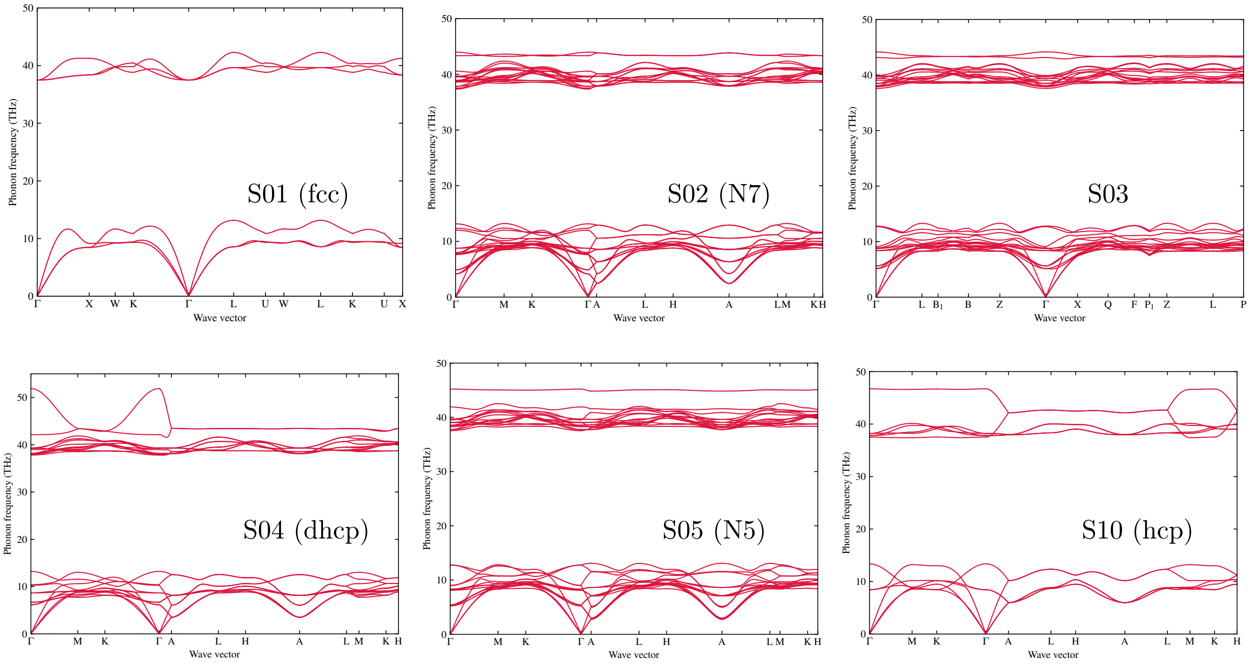


## 2.11 P= 100 GPa

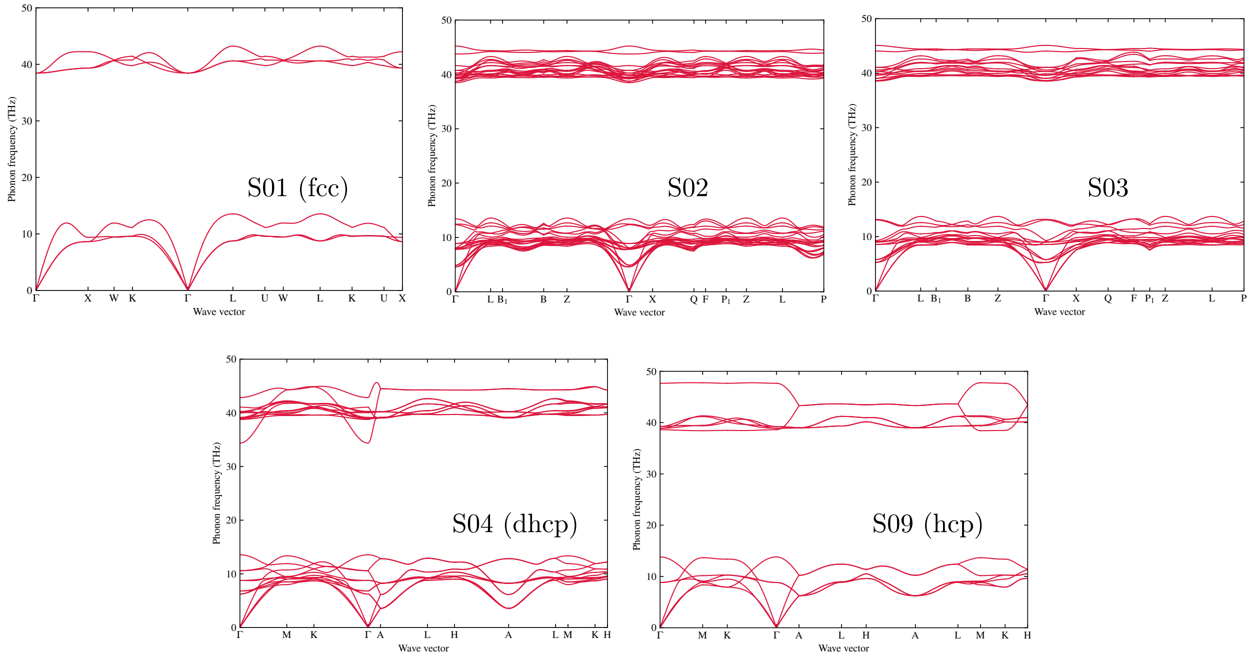

# 3 Phase diagram

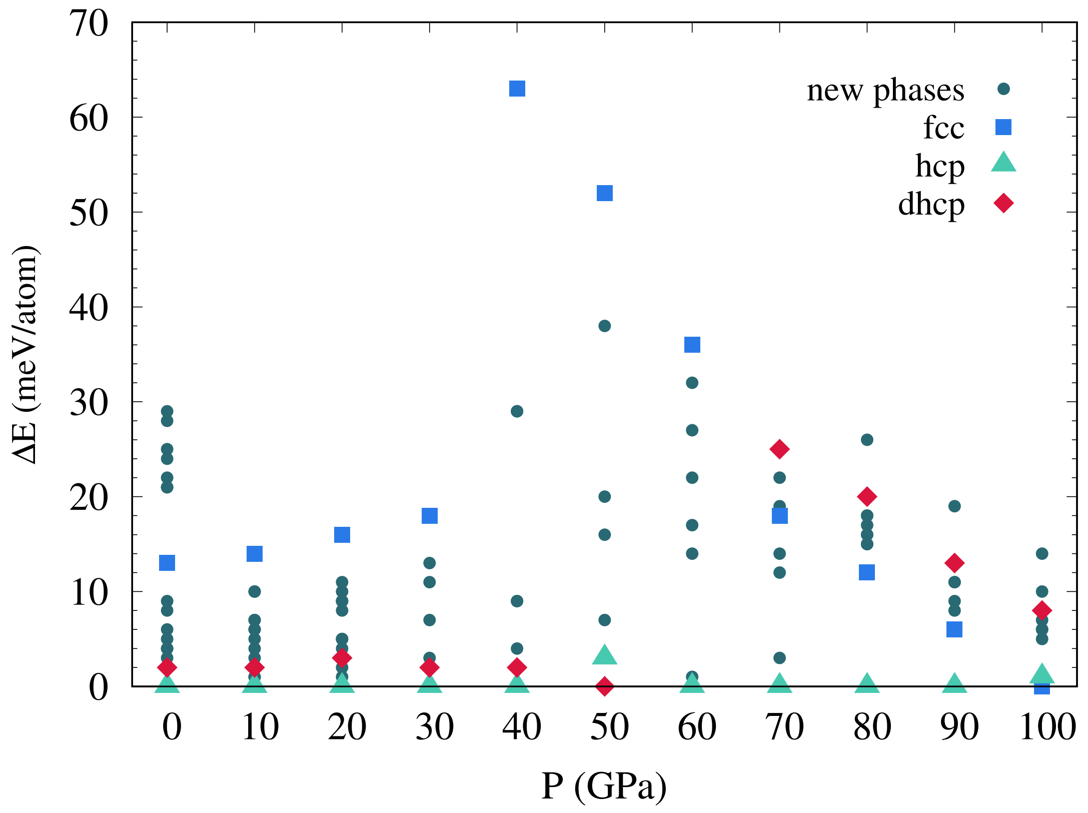


Figure S1: Relative energies as a function of pressure for the Fe-H structures without considering the free-energy corrections.

# 4 Bulk modulus

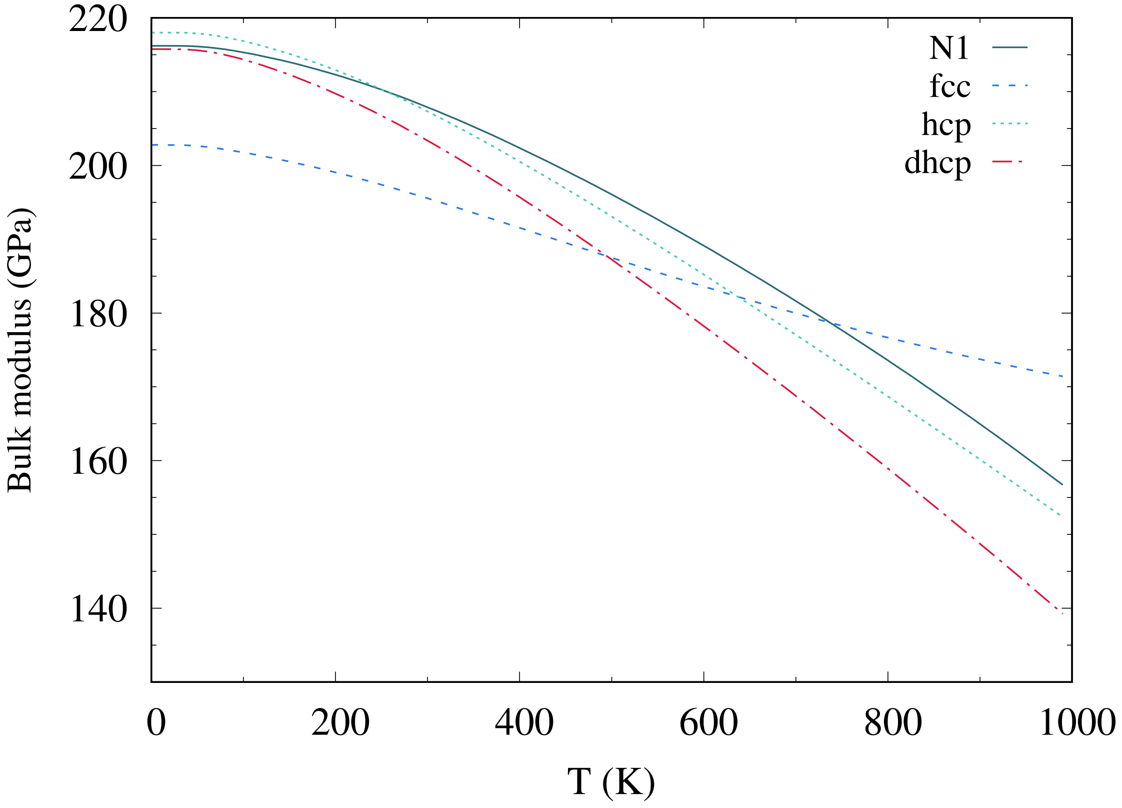


Figure S2: Bulk modulus as a function of temperature at 10 GPa for four different phases of FeH.

## 5 Electrical conductivity

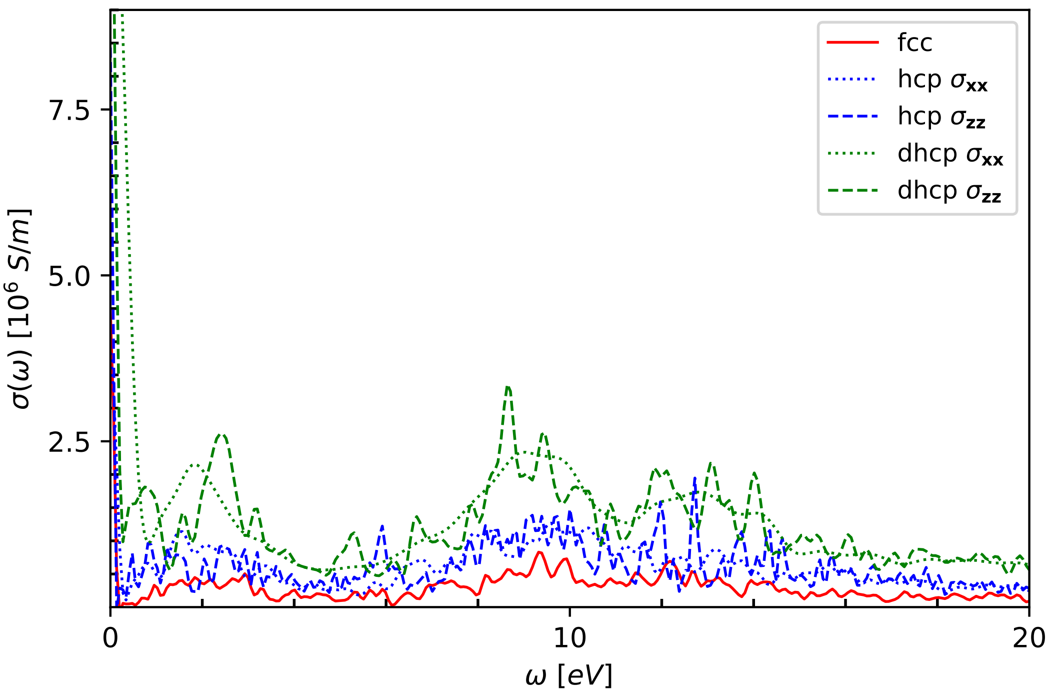


Figure S3: Frequency-dependent electrical conductivity of different phases of FeH at 0 GPa. Due to anisotropy, $\sigma_{\mathbf{xx}}$ and $\sigma_{\mathbf{zz}}$ components shown for *hcp* and *dhcp* phases.
